# Supplementary material for: Radiative Carrier Lifetime in Ge$_{1-x}$Sn$_x$ Mid-Infrared Emitters
Source: arXiv:2302.02467 ancillary file (2023-02-09)
Supplement: Supplementary file 1 [file Supplemental-material.pdf]

# Radiative Carrier Lifetime in GeSn Mid-Infrared Emitters

Gérard Daligou,[1] Anis Attiaoui,[1] Simone Assali,[1]
Patrick Del Vecchio,[1] and Oussama Moutanabbir[1,*]

[1]*Department of Engineering Physics, École Polytechnique de Montréal, C.P. 6079, Succ. Centre-Ville, Montréal, Québec, Canada H3C 3A7*

## Contents

S1. The momentum matrices and the eight-bands $k.p$ formalism 2

S2. Special-lines approximation 4

S3. Evolution of the bimolecular recombination coefficient with the excess carrier concentration $\Delta n$ 6

References 7

* oussama.moutanabbir@polymtl.ca

## S1. The momentum matrices and the eight-bands *k.p* formalism

The optical momentum matrix element in a bulk semiconductor is usually considered independent of the wave vector $\vec{k}$, and the polarization of the electromagnetic field. This isotropy is expressed by replacing the momentum matrix elements $M_{cv}^2(\vec{k})$ involved in the computation of $r^{\mathrm{sp}}$ with their average over the solid angle $d\Omega$ (see section 9.5 and appendix 9A of [2] for more information about the process). Herein, these matrix elements are computed from the eight-band $k.p$ Hamiltonian as discussed by Szmulowicz [9]. Several notations have been introduced to simplify the expressions of the different momentum matrices. Indeed, we denote by $\gamma_1', \gamma_2', \gamma_3'$ the modified Luttinger parameters for the eight bands $k.p$ model, and consider the notations

$$\Gamma_\pm = \gamma_2' \pm \gamma_1', \quad k_\pm = k_x \pm i k_y, \quad \eta_\pm(a,b) = \gamma_2' k_a \pm i\gamma_3' k_b$$

$$\alpha(x) = -\beta(x) = -1, \quad \alpha(y) = \beta(y) = i, \quad l(x) = -l(y) = 1$$

$$\rho(x) = \eta_+(x,y), \quad \rho(y) = \eta_-(y,x), \quad \chi(x) = \eta_-(x,y), \quad \chi(y) = \eta_+(y,x)$$

The impact of the coupling parameter $P$ on the conduction band Hamiltonian is highlighted by the parameter $A = \frac{\hbar^2}{2m_0} S$ with $S$, a dimensionless parameter given by equation (S1) where $m_e^*$ is the experimentally determined conduction band effective mass at the $\Gamma$ point, and $E_g$ is the unstrained bandgap energy [1].

$$S = \frac{m_0}{m_e^*} - \frac{2m_0}{\hbar^2}\left(\frac{E_g + \frac{2}{3}\Delta_{so}}{E_g(E_g + \Delta_{so})}\right)P^2. \tag{S1}$$

For bulk material grown on a (001) oriented substrate, in the angular momentum basis $\{|S\uparrow\rangle, |S\downarrow\rangle, |HH\uparrow\rangle, |LH\uparrow\rangle, |LH\downarrow\rangle, |HH\downarrow\rangle, |SO\uparrow\rangle, |SO\downarrow\rangle\}$[3], we have the matrices $M_x$, $M_y$ and $M_z$ as described by equations (S2) and (S3). Fig. S1 presents the polarization dependence of the strength of the different optical transitions between the conduction and the valence bands for the as-grown $Ge_{0.83}Sn_{0.17}$ layer. The wave vector $\vec{k}$ varies along the [100] direction. Fig. S1(a) and Fig. S1(b) present the contributions from the transverse electric (TE) polarization, and the the transverse magnetic (TM) polarization, respectively. A clear polarization dependence can be deduced through these figures. In fact, in the vicinity the $\Gamma$ point, the TE polarization promotes the transition from the conduction band to the heavy holes valence band. It is completely the opposite to the TM polarization for which this same transition is shown to be the least probable. At the same time, the wave vector $\vec{k}$ is shown to have a clear impact of the type of transition involved

in the computation of $r^{\mathrm{sp}}$, at least along the [100] direction. Fig. S2 presents the impact of the directions followed by $\vec{\boldsymbol{k}}$ in the Brillouin zone (BZ) on the interband transition strengths. Indeed, the evolution of the momentum matrix elements with $\vec{\boldsymbol{k}}$ is presented for the [100], [110], and [111] directions. Rather than comparing the transverse electric (TE) and the transverse magnetic (TM) separately, the average of the polarizations $(2 \times \mathrm{TE} + \mathrm{TM})/3$ is studied.

$$M(a) = \begin{pmatrix}
2Ak_a & 0 & -\frac{P\beta(a)}{\sqrt{2}} & 0 & -\frac{P\alpha(a)}{\sqrt{6}} & 0 & 0 & \frac{P\alpha(a)}{\sqrt{3}} \\
0 & 2Ak_a & 0 & -\frac{P\beta(a)}{\sqrt{6}} & 0 & -\frac{P\alpha(a)}{\sqrt{2}} & \frac{P\beta(a)}{\sqrt{3}} & 0 \\
\frac{P\alpha(a)}{\sqrt{2}} & 0 & -\frac{\hbar^2 k_a \Gamma_+}{m_0} & -\frac{\hbar^2 \alpha(a)\gamma_3' k_z \sqrt{3}}{m_0} & \frac{\hbar^2 l(a)\chi(a)\sqrt{3}}{m_0} & 0 & \frac{\hbar^2 \alpha(a)\gamma_3' k_z \sqrt{6}}{2m_0} & -\frac{\hbar^2 l(a)\chi(a)\sqrt{6}}{m_0} \\
0 & \frac{P\alpha(a)}{\sqrt{6}} & \frac{\hbar^2 \beta(a)\gamma_3' k_z \sqrt{3}}{m_0} & \frac{\hbar^2 k_a \Gamma_-}{m_0} & 0 & \frac{\hbar^2 l(a)\chi(a)\sqrt{3}}{m_0} & -\frac{\hbar^2 \sqrt{2}\gamma_2' k_a}{m_0} & -\frac{3\hbar^2 \alpha(a)\gamma_3' k_z \sqrt{2}}{2m_0} \\
\frac{P\beta(a)}{\sqrt{6}} & 0 & \frac{\hbar^2 l(a)\rho(a)\sqrt{3}}{m_0} & 0 & \frac{\hbar^2 k_a \Gamma_-}{m_0} & \frac{\hbar^2 \alpha(a)\gamma_3' k_z \sqrt{3}}{m_0} & \frac{3\hbar^2 \beta(a)\gamma_3' k_z \sqrt{2}}{2m_0} & \frac{\hbar^2 \sqrt{2}\gamma_2' k_a}{m_0} \\
0 & \frac{P\beta(a)}{\sqrt{2}} & 0 & \frac{\hbar^2 l(a)\rho(a)\sqrt{3}}{m_0} & -\frac{\hbar^2 \beta(a)\gamma_3' k_z \sqrt{3}}{m_0} & -\frac{\hbar^2 k_a \Gamma_+}{m_0} & \frac{\hbar^2 l(a)\rho(a)\sqrt{6}}{m_0} & -\frac{\hbar^2 \beta(a)\gamma_3' k_z \sqrt{6}}{2m_0} \\
0 & \frac{P\alpha(a)}{\sqrt{3}} & -\frac{\hbar^2 \beta(a)\gamma_3' k_z \sqrt{6}}{2m_0} & -\frac{\hbar^2 \sqrt{2}\gamma_2' k_a}{m_0} & -\frac{3\hbar^2 \alpha(a)\gamma_3' k_z \sqrt{2}}{2m_0} & \frac{\hbar^2 l(a)\chi(a)\sqrt{6}}{m_0} & -\frac{\hbar^2 \gamma_1' k_a}{m_0} & 0 \\
\frac{P\beta(a)}{\sqrt{3}} & 0 & -\frac{\hbar^2 l(a)\rho(a)\sqrt{6}}{m_0} & \frac{3\hbar^2 \beta(a)\gamma_3' k_z \sqrt{2}}{2m_0} & \frac{\hbar^2 \sqrt{2}\gamma_2' k_a}{m_0} & \frac{\hbar^2 \alpha(a)\gamma_3' k_z \sqrt{6}}{2m_0} & 0 & -\frac{\hbar^2 \gamma_1' k_a}{m_0}
\end{pmatrix} \tag{S2}$$

$$M_z = \begin{pmatrix}
2Ak_z & 0 & 0 & \sqrt{\frac{2}{3}}P & 0 & 0 & -\frac{P}{\sqrt{3}} & 0 \\
0 & 2Ak_z & 0 & 0 & \sqrt{\frac{2}{3}}P & 0 & 0 & \frac{P}{\sqrt{3}} \\
0 & 0 & -\frac{\hbar^2 k_z(\gamma_1' - 2\gamma_2')}{m_0} & \frac{\hbar^2 \sqrt{3}\gamma_3' k_-}{m_0} & 0 & 0 & -\frac{\hbar^2 \sqrt{6}\gamma_3' k_-}{2m_0} & 0 \\
\sqrt{\frac{2}{3}}P & 0 & \frac{\hbar^2 \sqrt{3}\gamma_3' k_+}{m_0} & -\frac{\hbar^2 k_z(\gamma_1' + 2\gamma_2')}{m_0} & 0 & 0 & \frac{2\hbar^2 \sqrt{2}\gamma_2' k_z}{m_0} & \frac{3\hbar^2 \sqrt{2}\gamma_3' k_-}{2m_0} \\
0 & \sqrt{\frac{2}{3}}P & 0 & 0 & -\frac{\hbar^2 k_z(\gamma_1' + 2\gamma_2')}{m_0} & -\frac{\hbar^2 \sqrt{3}\gamma_3' k_-}{m_0} & \frac{3\hbar^2 \sqrt{2}\gamma_3' k_+}{2m_0} & -\frac{2\hbar^2 \sqrt{2}\gamma_2' k_z}{m_0} \\
0 & 0 & 0 & 0 & -\frac{\hbar^2 \sqrt{3}\gamma_3' k_+}{m_0} & -\frac{\hbar^2 k_z(\gamma_1' - 2\gamma_2')}{m_0} & 0 & -\frac{\hbar^2 \sqrt{6}\gamma_3' k_+}{2m_0} \\
-\frac{P}{\sqrt{3}} & 0 & -\frac{\hbar^2 \sqrt{6}\gamma_3' k_+}{2m_0} & \frac{2\hbar^2 \sqrt{2}\gamma_2' k_z}{m_0} & \frac{3\hbar^2 \sqrt{2}\gamma_3' k_-}{2m_0} & 0 & -\frac{\hbar^2 \gamma_1' k_z}{m_0} & 0 \\
0 & \frac{P}{\sqrt{3}} & 0 & \frac{3\hbar^2 \sqrt{2}\gamma_3' k_+}{2m_0} & -\frac{2\hbar^2 \sqrt{2}\gamma_2' k_z}{m_0} & -\frac{\hbar^2 \sqrt{6}\gamma_3' k_-}{2m_0} & 0 & -\frac{\hbar^2 \gamma_1' k_z}{m_0}
\end{pmatrix} \tag{S3}$$

$M_x = M(x)$, $M_y = M(y)$

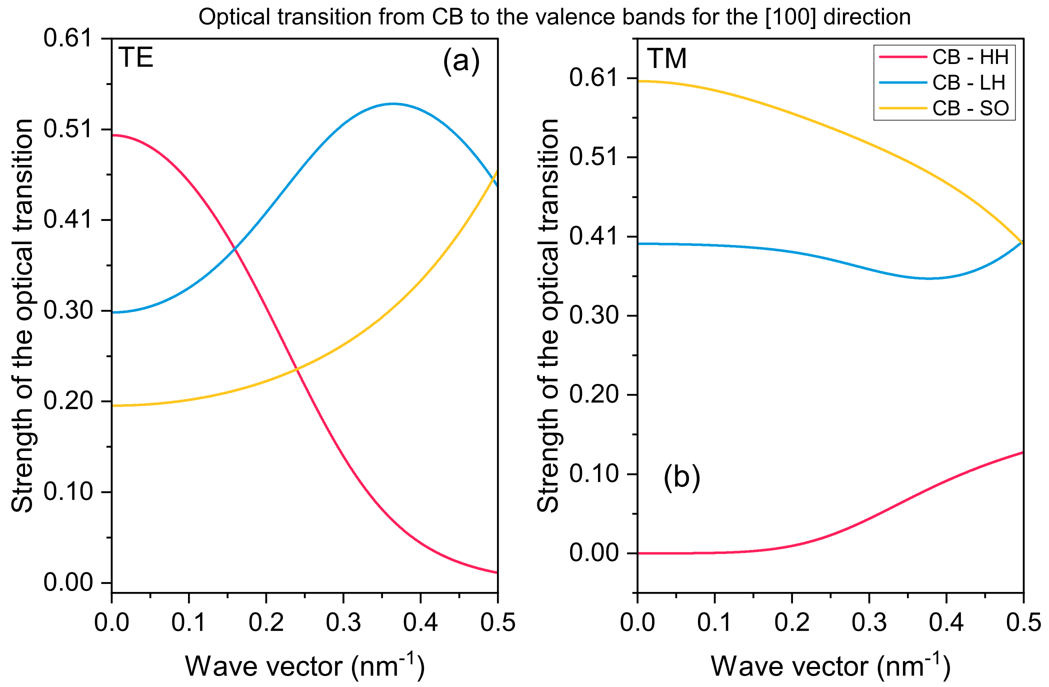


Figure S1. Strength of the transitions between the conduction and valence bands for the as-grown $Ge_{0.83}Sn_{0.17}$ at T = 4 K. Here, the wave vector $\vec{k}$ is along the [1 0 0] direction. The contribution from the transverse electric (TE) polarization is found using $\hat{\varepsilon} = (1, 0, 0)$ in equation (2) in the main text. For the transverse magnetic (TM), $\hat{\mathbf{e}} = (0, 0, 1)$. The strength presented here are normalized by $P^2$ with $P$ the Kane parameter.

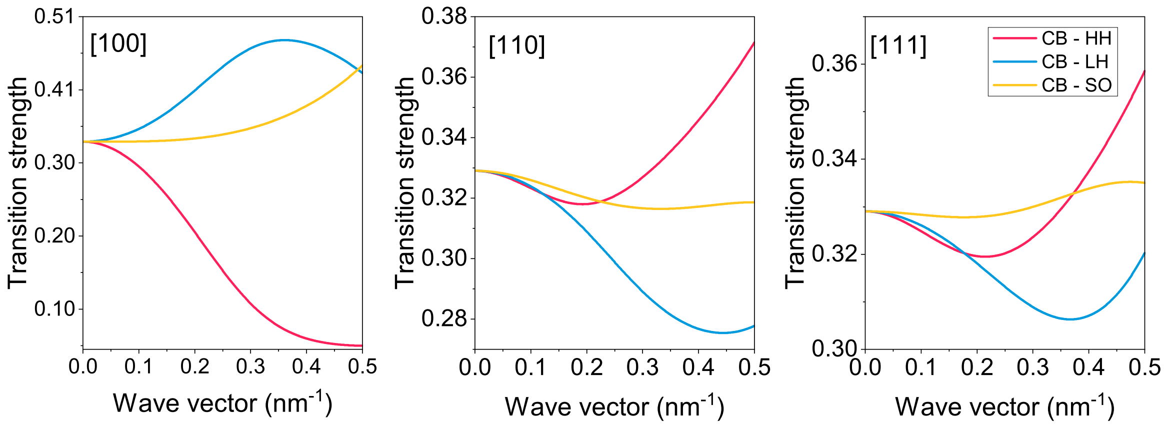


Figure S2. Comparison of the unpolarized optical strengths of the transitions between the conduction and valence bands for the as-grown $Ge_{0.83}Sn_{0.17}$ at T = 4 K. The unpolarized strengths are defined following the formula $(2M^2_{\mathrm{cv,TE}} + M^2_{\mathrm{cv,TM}})/3$

## S2. Special-lines approximation

For group IV semiconductors, the characteristic directions in the special-lines approximation (SLA) can be considered as [100], [110], and [111] with all their degeneracies ([100] six-fold, [110]

twelve-fold, and [111] eight-fold) included. In that case, the set of special directions should be

$$\begin{aligned}\mathcal{L} = \; &\{[100],[001],[010],[\bar{1}00],[0\bar{1}0],[00\bar{1}],[110],[101],[1\bar{1}0],\\ &[10\bar{1}],[\bar{1}10],[\bar{1}01],[\bar{1}\bar{1}0],[\bar{1}0\bar{1}],[011],[0\bar{1}\bar{1}],[0\bar{1}1],[01\bar{1}],\\ &[111],[11\bar{1}],[1\bar{1}1],[1\bar{1}\bar{1}],[\bar{1}\bar{1}\bar{1}],[\bar{1}11],[\bar{1}\bar{1}1],[\bar{1}1\bar{1}]\;\}\end{aligned} \quad \text{(S4)}$$

with a weight of 1/26 for each direction. Some of the directions are expected to be equivalent depending on the strain applied to the material. For example, for an unstrained material, $\mathcal{L}$ can be reduced to $\{[100],[110],[111]\}$ since [100], [110] and, [111] are equivalent to their degeneracies.

The symmetric directions are usually assumed to carry all the relevant sets of information. This assumption is not always accurate since less symmetric lines can also convey relevant details about the material. Therefore, more directions have to be considered in addition to the ones from equation (S4). In our model, the Kane's Y stars were considered to account for this specific case [5]. The Y stars are the $\vec{\boldsymbol{k}}$-directions forming equal angles with adjacent symmetry directions. There are forty-eight directions as presented in table 1 and figure 1 of [4]. With these new directions included, the set $\mathcal{L}$ from equation (S4) should have seventy-four elements. This increase of the number of characteristic directions involved would improve the accuracy of the computation of the integrals over the BZ, but also increase the computation time depending on the algorithm used. A trade-off should therefore be found between the accuracy of the computation and the computation time. For the as-grown $Ge_{0.83}Sn_{0.17}$ material, the seventy-four characteristic lines previously mentioned were found to be grouped into eight main classes, as shown in Fig. S3, highlighting the band structure of the as-grown material following different directions of the wave vector $\vec{\boldsymbol{k}}$.

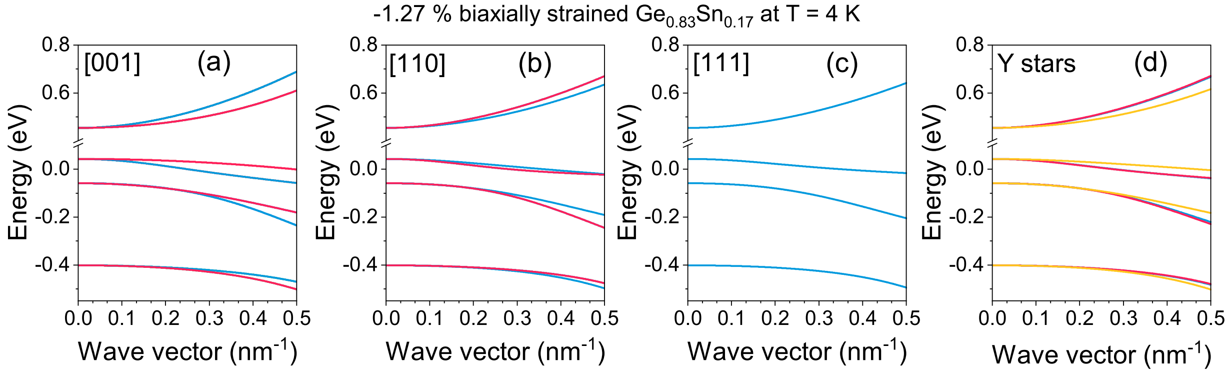


Figure S3. Determination of the characteristic directions considered within the special-lines approximation for the computation of the integrals over the Brillouin zone for a -1.27 % biaxially strained $Ge_{0.83}Sn_{0.17}$.

Fig. S3(a) presents the clustering of the [100] six degeneracies into two main classes. Indeed, the

[100] direction becomes four-fold degenerated while the [001] is now two-fold. It is also the case for [110] that is now four-fold degenerated while [101] is eight-fold. Regarding the [111] direction, only one class is obtained as presented in Fig. S3(c). As for the Y stars, Fig. S3(d) highlights only three lines, each of them sixteen-fold degenerated. The set $\mathcal{L}$ can therefore be reduced to

$$\mathcal{L} = \Big\{[100], [001], [110], [101], [111], [1, \sqrt{2}-1, \sqrt{3}-\sqrt{2}], \\ [1, \sqrt{3}-\sqrt{2}, \sqrt{2}-1], [\sqrt{3}-\sqrt{2}, \sqrt{2}-1, 1]\ \Big\} \tag{S5}$$

## S3. Evolution of the bimolecular recombination coefficient with the excess carrier concentration $\Delta n$

The bimolecular recombination coefficient $B$, presented in Fig. S4, is computed from the values of $R_{\mathrm{sp}}$ and $\Delta n$ extracted from the power-dependent photoluminescence (PL) spectra.

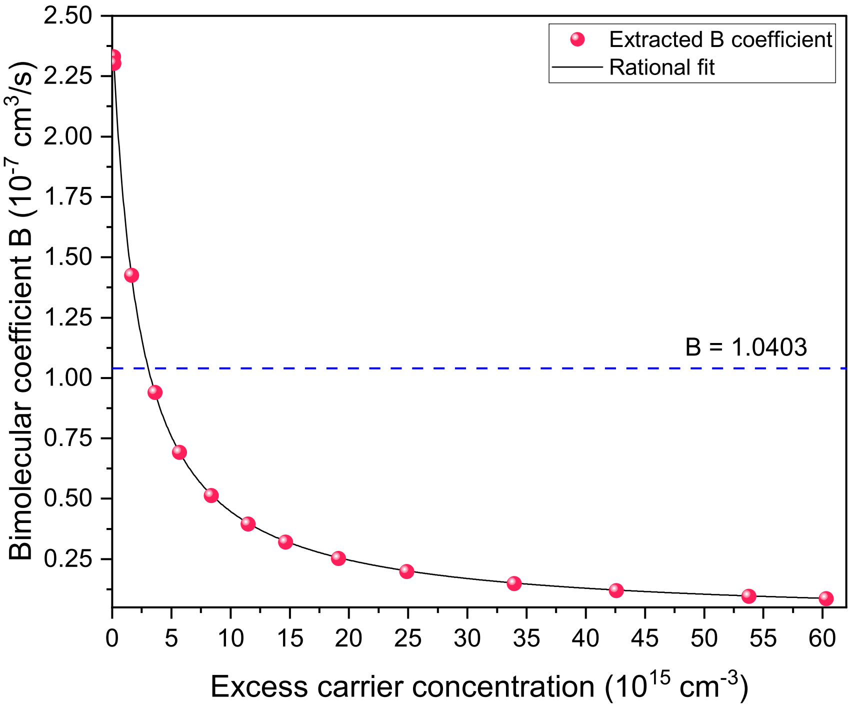


Figure S4. Extracted B coefficient from the fitting process of the 4 K power-dependent photoluminescence for the -1.27% biaxially strained $Ge_{0.83}Sn_{0.17}$.

Rather than being constant, it decreases with $\Delta n$, as suggested earlier for III-V semiconductors [7, 8]. However, its evolution for the as-grown $Ge_{0.83}Sn_{0.17}$ is not as linear as presented by Olshansky et al. for InGaAsP and AlGaAs light sources [6]. Using a rational function, the evolution of the

bimolecular recombination coefficient $B$ extracted from the experimental results was fitted, resulting in equation (S6) with $B_0 = (-7.792 \pm 7.225) \times 10^{-10}\,\mathrm{cm}^{-3}\,\mathrm{s}^{-1}$, $B_1 = (3.783 \pm 0.161) \times 10^{-22}\,\mathrm{s}^{-1}$, $B_2 = (1.523 \pm 0.030) \times 10^{-15}\,\mathrm{cm}^{-3}$, and $B_3 = (6.932 \pm 2.210) \times 10^{-31}$.

$$B = \frac{B_0 + B_1 \Delta n}{B_2 \Delta n + B_3 (\Delta n)^2} \tag{S6}$$

On top of that, the value extracted at $\Delta n = 6 \times 10^{16}\,\mathrm{cm}^{-3}$ is two orders of magnitude lower than the value of $1.04 \times 10^{-7}\,\mathrm{cm}^3/\mathrm{s}$ computed assuming parabolic band dispersion and non-degenerate semiconductor.


[1] Stefan Birner. *Modeling of Semiconductor Nanostructures and Semiconductor-Electrolyte Interfaces*. Number vol. 135 in Selected Topics of Semiconductor Physics and Technology. Verein zur Förderung des Walter Schottky Instituts der Technischen Universität München, 1. aufl edition, 2011.

[2] Shun Lien Chuang. *Physics of Photonic Devices*. Wiley Series in Pure and Applied Optics. Wiley, 2. ed edition, 2009.

[3] Thomas Eißfeller. *Theory of the Electronic Structure of Quantum Dots in External Fields*. Number Vol. 146 in Selected Topics of Semiconductor Physics and Technology. Verein zur Förderung des Walter-Schottky-Inst. der Techn. Univ. München, 1. aufl edition, 2012.

[4] P Enders. Addendum to 'Special-lines approximation to Brillouin zone integration': Improved set of special lines. *Semiconductor Science and Technology*, 11(12):1927–1929, 1996.

[5] E.O. Kane. Energy band structure in p-type germanium and silicon. *Journal of Physics and Chemistry of Solids*, 1(1-2):82–99, 1956.

[6] R. Olshansky, C. Su, J. Manning, and W. Powazinik. Measurement of radiative and nonradiative recombination rates in ingaasp and algaas light sources. *IEEE Journal of Quantum Electronics*, 20(8):838–854, 1984.

[7] Frank Stern. Calculated spectral dependence of gain in excited GaAs. *Journal of Applied Physics*, 47(12):5382–5386, 1976.

[8] C. B. Su, R. Olshansky, J. Manning, and W. Powazinik. Carrier dependence of the radiative coefficient in III-V semiconductor light sources. *Applied Physics Letters*, 44(8):732–734, 1984.

[9] Frank Szmulowicz. Derivation of a general expression for the momentum matrix elements within the envelope-function approximation. *Physical Review B*, 51(3):1613–1623, 1995.
